# Supplementary material for: Noisy defects in a doped Mott insulator
Source: arXiv:1809.09840 ancillary file (2018-09-26)
Supplement: Supplementary file 1 [file Supplementary_Information.pdf]

# Supplementary Information to ‘Noisy defects in a doped Mott insulator’

F. Massee, Y. K. Huang & M. Aprili

## 1 Dopant location

In line with previous reports<sup>1-3</sup>, we find resonant states associated with oxygen dopants at  $E = -1$  V and  $E = -1.5$  eV, as displayed in Fig. S1. The position of the  $E = -1$  eV states is in between four neighbouring Bi atoms, whereas the  $E = -1.5$  eV states are in between two Bi atoms. Calculations have shown that the strongest intensity for the  $E = -1.5$  eV resonance should be located away from the centre of the defect along the direction of the nearest neighbour Bi atoms<sup>3</sup>, leading to two differently oriented resonances depending on the position of the dopant in the unit cell. Unlike previous efforts, we in fact resolve such anisotropic resonances with two possible orientations as can be seen in Fig. S1b. The enlargement of one of the near-horizontally oriented states in the inset of Fig. S1b clearly shows the directionality of the highest density of states along the nearest neighbour Bi atoms.

In addition to these previously detected resonant states, we find additional states at a range of energies  $< -500$  meV. Unlike the known resonant states, these additional states show enhanced current noise. To visualize that these noisy defects are different from the  $E = -1$  eV and  $E = -1.5$  eV states, we plot the Fano image of the main text with the positions of the two types of standard resonances in Fig. S1c: the noisy defects do not coincide with the known dopants.

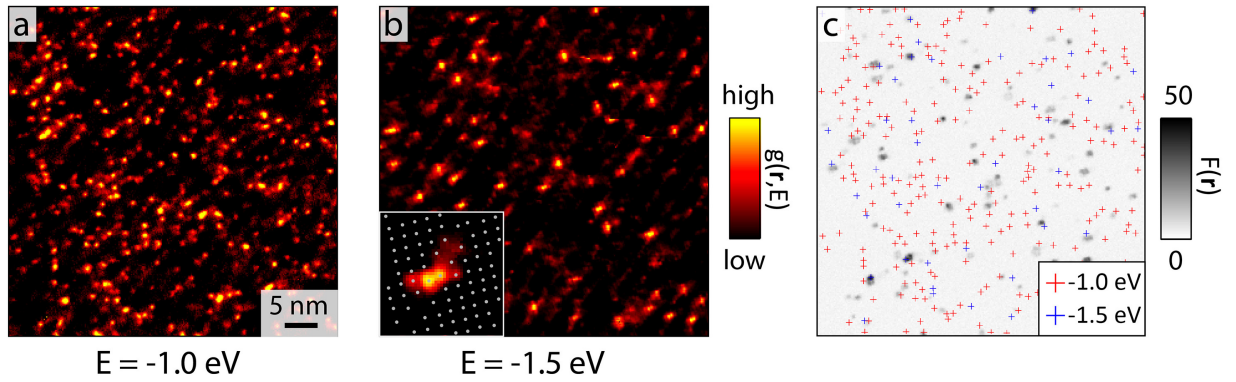

**Figure S1 Oxygen dopant location.** **a,b** Differential conductance,  $g(r, E)$ , at -1 eV and -1.5 eV, respectively. In the latter, the defects are oriented either near-horizontal or near-vertical. The inset of **b** shows a single near-horizontal defect state with the atomic (Bi) positions indicated with white dots. **c** Fano image ( $E = -1.5$  eV and  $I = 400$  pA) taken at the same location as **a,b**. The noisy defects do not coincide with the known oxygen defects.

## 2 Noise and differential conductance

The current noise and differential conductance are strongly linked to one another as is evident from the point spectrum shown in the main text Fig. 2c. However, the noise gives us a deeper insight into the mechanism underlying changes in the differential conductance that spectroscopy in itself cannot provide. To show how strongly linked the two observables are, not only in energy, but also spatially, we display in Fig. S2 differential conductance images simultaneously taken with Fano images in the area encompassing that shown in Fig. 3 of the main text. From these images it is immediately evident that the differential conductance and the excess current noise are strongly linked both in energy and location.

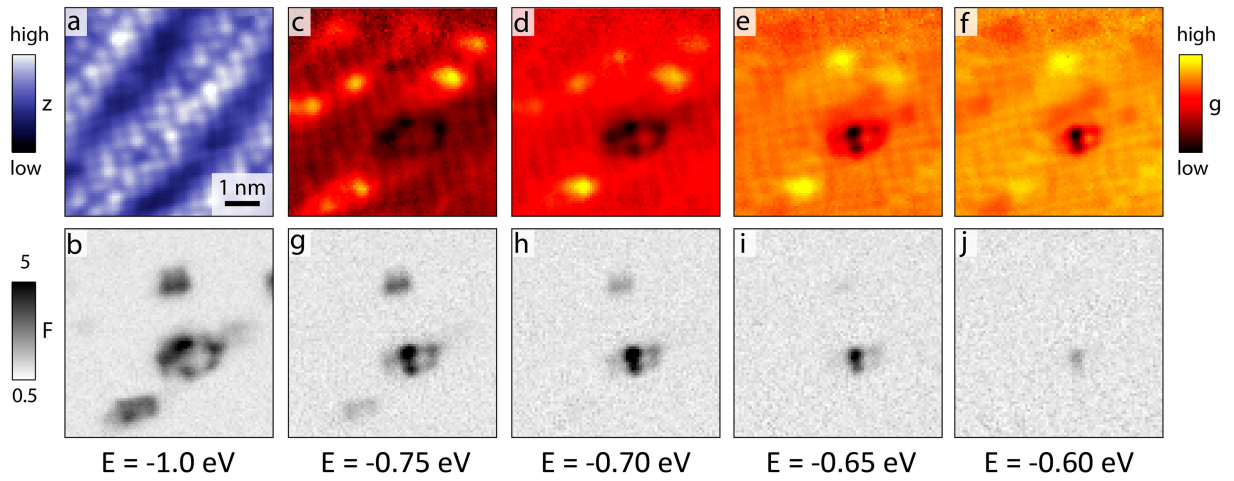

**Figure S2 Strong link between  $dI/dV$  and current noise.** **a** Constant current image at  $E = -1$  eV and  $I = 500$  pA. **b** Fano image at the setup energy and current of **a**. **c-f** Differential conductance images at the same field of view as **a,b** showing a clearly dispersing signal. **g-j** Fano images simultaneously taken with the  $dI/dV$  image displayed above them, the energy of the Fano image and corresponding differential conductance image is indicated below the Fano images.

### 3 Current dependence of $dI/dV$

One important clue as to how oxygen dopant atoms, which are located at the same xy-location within experimental error, can lead to very different dynamics is found in the current dependence of the differential conductance. A distinct dependence on the current is a well-known characteristic of tip induced band bending<sup>4</sup>, the strength of which depends crucially on the depth of the defect. The defect in Fig. 3 of the main text shows a very strong current dependence, suggesting it is located rather close to the top BiO plane. In general, the differential conductance of defects that show enhanced current noise right above the defect position have a finite, but less pronounced current dependence - two examples are shown in Fig. S3a,b. The differential conductance of oxygen states without enhanced current noise do not show an observable current dependence, see Fig. S3c. The distance of a dopant atom from the BiO plane therefore seems to be an important factor in determining the coupling to the CuO charge reservoir that dictates the presence or absence of charge dynamics.

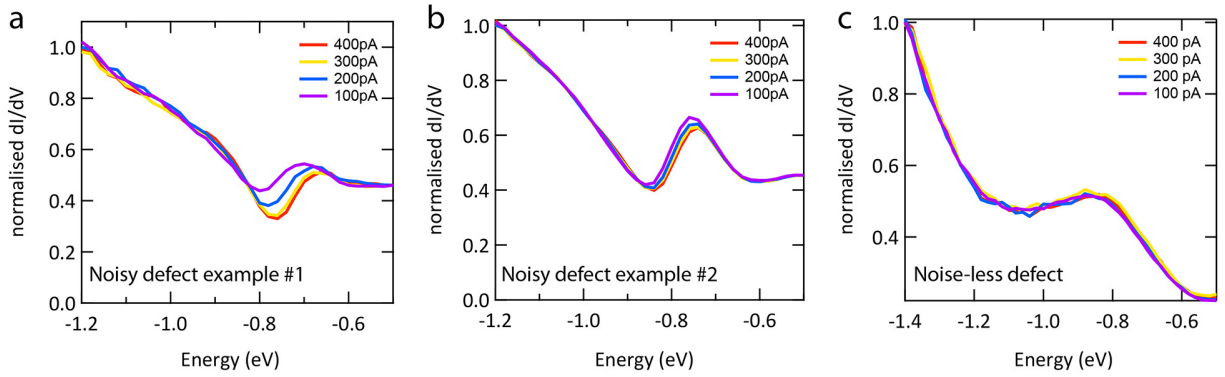

**Figure S3 Current dependence of  $dI/dV$ .** **a** Differential conductance recorded for increasing setup currents for a defects where the enhanced current noise is located in between four Bi atoms, i.e. right above the defect. **b** Another example of the current dependent  $dI/dV$  of a noisy defect with enhanced current noise directly above the defect. **c** Measurements on top of a Poissonian defect show no appreciable dependence on the current.

#### 4 Voltage dependence of Fano factor at $E > E_{\text{resonance}}$

In the presence of a modulating potential, the excess current noise will reflect the derivative of the differential conductance with respect to the potential fluctuation. In Fig. S4a,b we show the differential conductance and its numerical derivative, respectively. Due to the appearance of the CuO bands between  $E = -1$  eV and  $-1.5$  eV, the derivative of the differential conductance strongly increases. At energies above that of the resonance, instead of returning to the Poissonian value of  $F = 1$ , the Fano factor is seen to increase, mimicking the  $dI^2/dV^2$  in line with a modulating potential due to charge trapping and de-trapping at the dopant site.

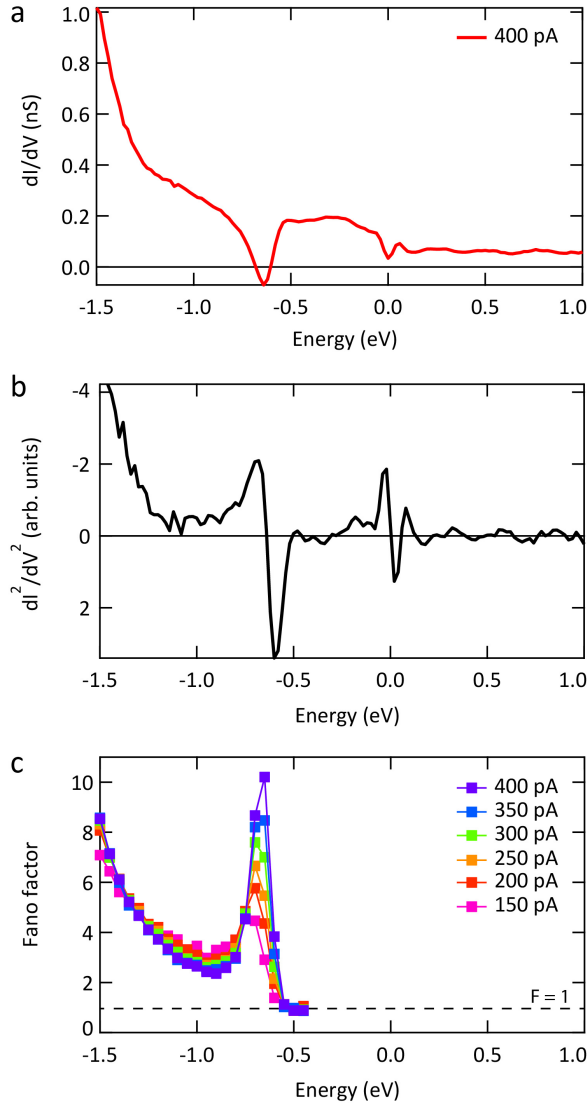

**Figure S4 Noise vs  $dI^2/dV^2$ .** **a** Differential conductance at the defect in Fig. 3 of the main text ( $E_{\text{setup}} = -1.5$  eV,  $I_{\text{setup}} = 400$  pA). **b** Numerical derivative of **a**. **c** Voltage dependence of the Fano factor for a range of currents. At energies above the resonant energy, the voltage dependence strongly mimics the derivative of the differential conductance.

## 5 Circuit and tip independence

To exclude that our observed noisy defects are artefacts due to the AC circuitry, or an unusual tip termination, we performed several tests. Firstly, we can completely disconnect our low temperature AC circuitry with a low temperature switch without altering the measurement conditions. When we do this at a location with negative differential conductance, like that shown in Fig. 3 of the main text, the negative differential conductance and its current dependence persists even without AC circuitry, see Fig. S5. We can therefore exclude that our circuitry affects our measured signal.

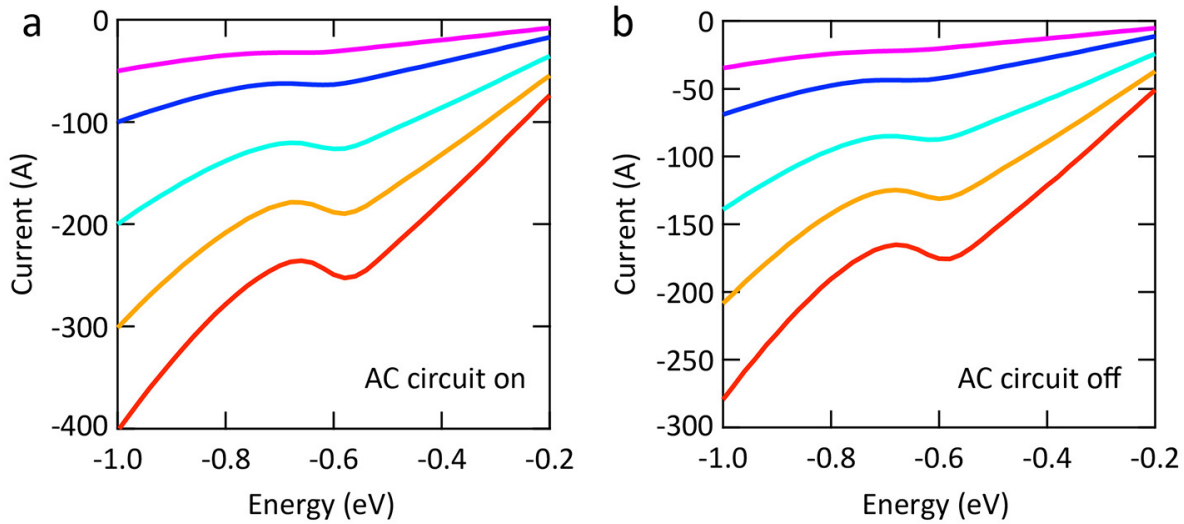

**Figure S5 AC circuit on/off.** **a** Negative resistance measured with AC circuitry for different setup currents on the defect shown in Fig. 3 of the main text ( $E_{\text{setup}} = -1$  eV, **b**). **b** Spectra on the same location without AC circuitry ( $E_{\text{setup}} = -1.2$  eV), proving that the circuitry has no influence on the negative resistance (note that the current scale is different between **a** and **b** due to different set voltages).

To determine whether the excess current noise we observe is intrinsic to Bi2212 or somehow a tip effect, we intentionally blunted our tip. Figure S6a,b show the same field of view before and after blunting, respectively. There is still atomic contrast after tip indentation, but it is heavily blurred and double. The excess current noise, although reduced in amplitude, is still present (see Fig. 6c,d). Additionally, we find the same range of atomically sized defects with enhanced current noise on multiple samples, using different tips, made of a different tip material (W instead of Pt/Ir, see Fig. 6e,f). We therefore conclude that our observations are not a measurement artefact, but intrinsic properties of tunnelling into Bi2212.

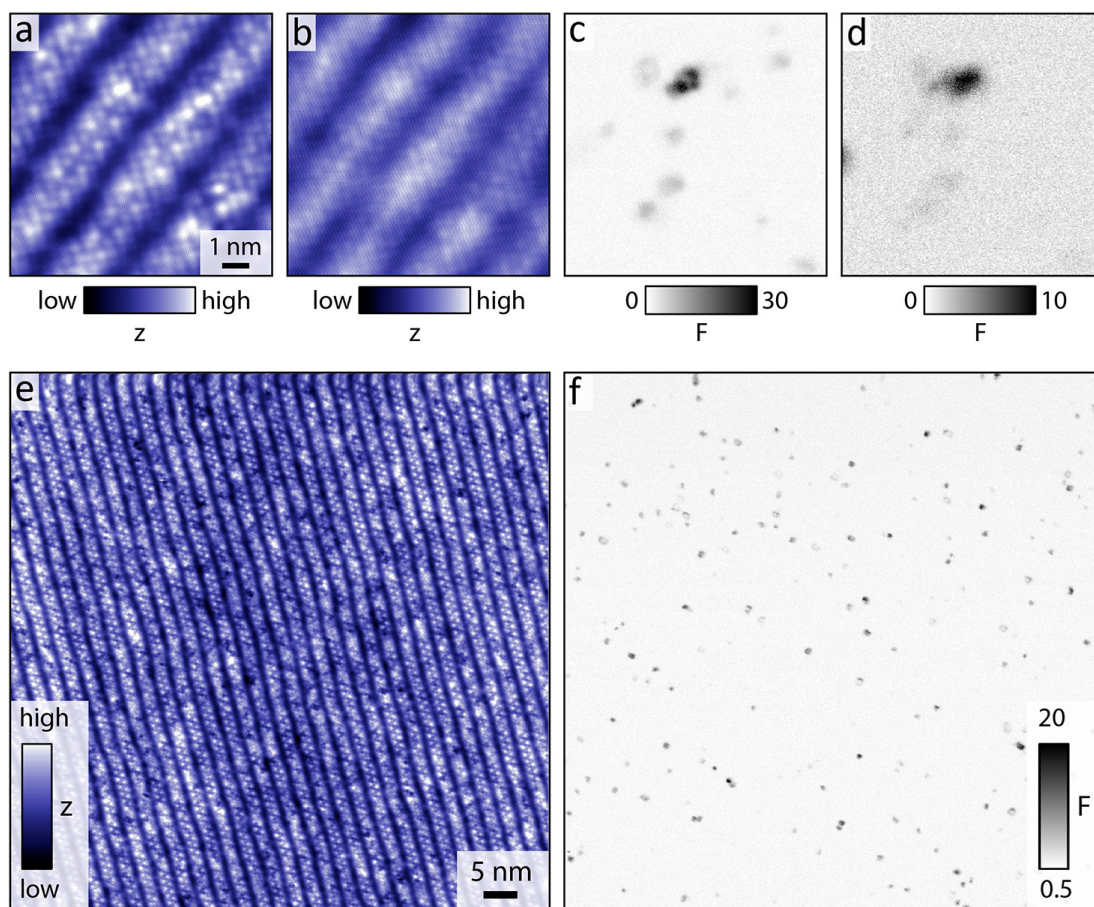

**Figure S6 Tip.** **a,b** Constant current images on the same field of view with a sharp and blunt tip respectively ( $E = -1.5$  eV,  $I = 400$  pA). **c,d** Fano images corresponding to **a,b**. Although the contrast is blurred with the blunt tip, the excess current noise is still observed. **e,f** Constant current and Fano image ( $E = -1$  eV,  $I = 400$  pA), respectively, using a W tip on a different sample cleave, showing the same behaviour as with the Pt/Ir tip presented throughout the main text.

## References

1. K. McElroy et al., Science **309**, 1048 (2005)
2. I. Zeljkovic et al., Science **337**, 320 (2012)
3. I. Zeljkovic et al., Nano Letters **14**, 6749 (2014)
4. R. M. Feenstra and J. A. Stroscio, J. Vac. Sci. Technol. B **5**, 923 (1987)
